# Supplementary material for: E2S2: Encoding-Enhanced Sequence-to-Sequence Pretraining for Language Understanding and Generation
Source: arXiv:2205.14912 source file (2024-01-09)
Supplement: Supplementary file 1 [file appendix.tex]

\appendix
\section{Appendix}
\input{hyper_parameters.tex}
% \paragraph{Appendix}
\subsection{Details of Tasks in GLUE benchmark}
\label{appendix_data}
As mentioned in Section~\ref{sec:experiment}, we conduct extensive experiments on GLUE benchmarks for evaluating the performance on language understanding. Here, we introduce the descriptions of tasks in GLUE benchmark in detail. Each task is described as:

\textbf{CoLA.} Corpus of Linguistic Acceptability~\cite{warstadt2019neural} is a binary single-sentence classification task to determine whether a given sentence is linguistically ``acceptable''.

\textbf{SST-2.} Stanford Sentiment Treebank~\cite{socher2013recursive} is a binary-classification task that aims to predict the sentiment of a given sentence from movie reviews.

\textbf{MRPC.} Microsoft Research Paraphrase Corpus~\cite{dolan2005automatically} is a task to predict whether two sentences automatically extracted from online news sources are semantically equivalent.

\textbf{STS-B.} Semantic Textual Similarity~\cite{cer2017semeval} is a task to predict how similar two sentences are on a 1-5 scale in terms of semantic meaning.

\textbf{MNLI.} Multi-Genre Natural Language Inference Corpus~\cite{williams2018broad} is a natural language inference task, which is to predict whether the premise entails the hypothesis, contradicts the hypothesis, or neither, given a premise sentence and a hypothesis sentence.

\textbf{QQP.} Quora Question Pairs dataset\footnote{\url{https://data.quora.com/First-Quora-Dataset-Release-Question-Pairs}} is a collection of question pairs from the community question-answering website Quora. The task is to determine whether a pair of questions are semantically equivalent. 

\textbf{QNLI.} Question Natural Language Inference is a binary classification task constructed from SQuAD~\cite{rajpurkar2016squad}, which aims to predict whether a context sentence contains the answer to a question sentence. 

\textbf{RTE.} Recognizing Textual Entailment~\cite{giampiccolo2007third}, given a premise and a hypothesis, is a task to predict whether the premise entails the hypothesis. 

\subsection{Hyper-parameters of Fine-tuning}
\label{appendix_parameters}
Here, we show the details of hyper-parameters for fine-tuning on each downsteam tasks, in Tab.~\ref{tab:setting}. Recall that we conduct all experiments using the fairseq toolkit.
